# Supplementary material for: Text2Layer: Layered Image Generation using Latent Diffusion Model
Source: arXiv:2307.09781 source file (2023-07-19)
Supplement: Supplementary file 1 [file appendix.tex]

\appendix
